# Supplementary material for: Long Range Propagation on Continuous-Time Dynamic Graphs
Source: arXiv:2406.02740 source file (2024-06-04)
Supplement: Supplementary file 4 [file appendix_time_vs_embedding_dim.tex]

% This table is just for reference. Instead of this we will make a plot
             &                time &  dim & nlayer &  params \\
DyRep        &   21.17$_{\pm0.14}$ &   10 &      1 &     4238 \\
DyRep        &   23.52$_{\pm0.23}$ &   50 &      1 &    35178 \\
DyRep        &   27.07$_{\pm0.32}$ &  100 &      1 &   105353 \\
DyRep        &    30.67$_{\pm0.3}$ &  150 &      1 &   210528 \\
DyRep        &   33.53$_{\pm0.22}$ &  200 &      1 &   350703 \\
JODIE        &   18.05$_{\pm0.25}$ &   10 &      1 &     2402 \\
JODIE        &    18.57$_{\pm0.2}$ &   50 &      1 &    19862 \\
JODIE        &   20.62$_{\pm0.24}$ &  100 &      1 &    59687 \\
JODIE        &   22.42$_{\pm0.18}$ &  150 &      1 &   119512 \\
JODIE        &   23.96$_{\pm0.13}$ &  200 &      1 &   199337 \\
TGAT         &    7.52$_{\pm0.09}$ &   10 &      1 &     4168 \\
TGAT         &    8.94$_{\pm0.09}$ &   50 &      1 &    24708 \\
TGAT         &   11.56$_{\pm0.14}$ &  100 &      1 &    59383 \\
TGAT         &   14.44$_{\pm0.21}$ &  150 &      1 &   104058 \\
TGAT         &   16.62$_{\pm0.25}$ &  200 &      1 &   158733 \\
TGAT         &   37.57$_{\pm0.21}$ &   10 &      5 &    26056 \\
TGAT         &   62.33$_{\pm0.13}$ &   50 &      5 &   261636 \\
TGAT         &  101.26$_{\pm0.46}$ &  100 &      5 &   853111 \\
TGAT         &   154.1$_{\pm0.71}$ &  150 &      5 &  1774586 \\
TGAT         &    203.3$_{\pm0.9}$ &  200 &      5 &  3026061 \\
TGN          &   20.61$_{\pm0.11}$ &   10 &      1 &    11568 \\
TGN          &   24.37$_{\pm0.21}$ &   50 &      1 &    95708 \\
TGN          &   30.92$_{\pm0.25}$ &  100 &      1 &   286383 \\
TGN          &    38.0$_{\pm0.25}$ &  150 &      1 &   572058 \\
TGN          &   45.56$_{\pm0.19}$ &  200 &      1 &   952733 \\
TGN          &   55.79$_{\pm0.28}$ &   10 &      5 &    33328 \\
TGN          &   83.44$_{\pm0.33}$ &   50 &      5 &   332508 \\
TGN          &   127.99$_{\pm0.6}$ &  100 &      5 &  1079983 \\
TGN          &  188.24$_{\pm0.62}$ &  150 &      5 &  2242458 \\
TGN          &  246.59$_{\pm1.77}$ &  200 &      5 &  3819933 \\
Our          &    7.93$_{\pm0.11}$ &   10 &      1 &     2698 \\
Our          &    9.03$_{\pm0.16}$ &   50 &      1 &    27358 \\
Our          &   11.22$_{\pm0.11}$ &  100 &      1 &    89683 \\
Our          &   17.63$_{\pm1.24}$ &  150 &      1 &   187008 \\
Our          &   17.66$_{\pm1.01}$ &  200 &      1 &   319333 \\
Our          &   29.78$_{\pm0.11}$ &   10 &      5 &     2698 \\
Our          &   41.78$_{\pm0.27}$ &   50 &      5 &    27358 \\
Our          &   60.19$_{\pm1.12}$ &  100 &      5 &    89683 \\
Our          &    87.04$_{\pm3.1}$ &  150 &      5 &   187008 \\
Our          &   109.2$_{\pm5.69}$ &  200 &      5 &   319333 \\
Our(tanh)    &    7.87$_{\pm0.11}$ &   10 &      1 &     2698 \\
Our(tanh)    &    8.97$_{\pm0.12}$ &   50 &      1 &    27358 \\
Our(tanh)    &   11.16$_{\pm0.11}$ &  100 &      1 &    89683 \\
Our(tanh)    &   14.42$_{\pm0.22}$ &  150 &      1 &   187008 \\
Our(tanh)    &   16.83$_{\pm0.17}$ &  200 &      1 &   319333 \\
Our(tanh)    &   29.82$_{\pm0.24}$ &   10 &      5 &     2698 \\
Our(tanh)    &   41.57$_{\pm0.26}$ &   50 &      5 &    27358 \\
Our(tanh)    &    60.16$_{\pm0.2}$ &  100 &      5 &    89683 \\
Our(tanh)    &   84.61$_{\pm0.32}$ &  150 &      5 &   187008 \\
Our(tanh)    &   103.63$_{\pm0.4}$ &  200 &      5 &   319333 \\

%% data for table 8 
DyRep            &  Wikipedia &      27.07$_{\pm0.32}$ &  100 &      1 &   105353 \\
DyRep            &     Reddit &     161.43$_{\pm0.96}$ &  100 &      1 &   105353 \\
DyRep            &     LastFM &     216.88$_{\pm2.83}$ &  100 &      1 &    71353 \\
DyRep            &       MOOC &      53.32$_{\pm0.56}$ &  100 &      1 &    71753 \\
JODIE            &  Wikipedia &      20.62$_{\pm0.24}$ &  100 &      1 &    59687 \\
JODIE            &     Reddit &     131.71$_{\pm0.85}$ &  100 &      1 &    59687 \\
JODIE            &     LastFM &     176.61$_{\pm3.02}$ &  100 &      1 &    42687 \\
JODIE            &       MOOC &      43.92$_{\pm0.68}$ &  100 &      1 &    42887 \\
TGAT$_{1L}$      &  Wikipedia &      11.56$_{\pm0.14}$ &  100 &      1 &    59383 \\
TGAT$_{1L}$      &     Reddit &      67.83$_{\pm0.64}$ &  100 &      1 &    59383 \\
TGAT$_{1L}$      &     LastFM &    139.79$_{\pm20.78}$ &  100 &      1 &    25383 \\
TGAT$_{1L}$      &       MOOC &       33.92$_{\pm0.5}$ &  100 &      1 &    25783 \\
TGAT$_{5L}$      &  Wikipedia &     101.26$_{\pm0.46}$ &  100 &      5 &   853111 \\
TGAT$_{5L}$      &     Reddit &     895.35$_{\pm5.46}$ &  100 &      5 &   853111 \\
TGAT$_{5L}$      &     LastFM &   862.47$_{\pm217.38}$ &  100 &      5 &   683111 \\
TGAT$_{5L}$      &       MOOC &      73.77$_{\pm1.29}$ &  100 &      5 &   685111 \\
TGN$_{1L}$       &  Wikipedia &      30.92$_{\pm0.25}$ &  100 &      1 &   286383 \\
TGN$_{1L}$       &     Reddit &     196.87$_{\pm1.35}$ &  100 &      1 &   286383 \\
TGN$_{1L}$       &     LastFM &    289.22$_{\pm30.38}$ &  100 &      1 &   201383 \\
TGN$_{1L}$       &       MOOC &      53.46$_{\pm0.62}$ &  100 &      1 &   202383 \\
TGN$_{5L}$       &  Wikipedia &      127.99$_{\pm0.6}$ &  100 &      5 &  1079983 \\
TGN$_{5L}$       &     Reddit &    1099.19$_{\pm3.91}$ &  100 &      5 &  1079983 \\
TGN$_{5L}$       &     LastFM &  1034.24$_{\pm221.04}$ &  100 &      5 &   858983 \\
TGN$_{5L}$       &       MOOC &      95.45$_{\pm1.07}$ &  100 &      5 &   861583 \\
Our$_{1L}$       &  Wikipedia &      11.22$_{\pm0.11}$ &  100 &      1 &    89683 \\
Our$_{1L}$       &     Reddit &      64.48$_{\pm0.56}$ &  100 &      1 &    89683 \\
Our$_{1L}$       &     LastFM &    123.19$_{\pm11.33}$ &  100 &      1 &    72683 \\
Our$_{1L}$       &       MOOC &      35.49$_{\pm0.56}$ &  100 &      1 &    72883 \\
Our$_{5L}$       &  Wikipedia &      60.19$_{\pm1.12}$ &  100 &      5 &    89683 \\
Our$_{5L}$       &     Reddit &     533.91$_{\pm6.07}$ &  100 &      5 &    89683 \\
Our$_{5L}$       &     LastFM &   495.18$_{\pm111.13}$ &  100 &      5 &    72683 \\
Our$_{5L}$       &       MOOC &      56.33$_{\pm0.82}$ &  100 &      5 &    72883 \\
Our(tanh)$_{1L}$ &  Wikipedia &      11.16$_{\pm0.11}$ &  100 &      1 &    89683 \\
Our(tanh)$_{1L}$ &     Reddit &       65.1$_{\pm1.12}$ &  100 &      1 &    89683 \\
Our(tanh)$_{1L}$ &     LastFM &    123.46$_{\pm11.39}$ &  100 &      1 &    72683 \\
Our(tanh)$_{1L}$ &       MOOC &       34.42$_{\pm0.5}$ &  100 &      1 &    72883 \\
Our(tanh)$_{5L}$ &  Wikipedia &       60.16$_{\pm0.2}$ &  100 &      5 &    89683 \\
Our(tanh)$_{5L}$ &     Reddit &   532.36$_{\pm9.87}$ &  100 &      5 &   89683\\      
Our(tanh)$_{5L}$ &     LastFM &   496.28$_{\pm112.68}$ &  100 &      5 &    72683 \\
Our(tanh)$_{5L}$ &       MOOC &      56.19$_{\pm0.63}$ &  100 &      5 &    72883 \\
