# Supplementary material for: Long Range Propagation on Continuous-Time Dynamic Graphs
Source: arXiv:2406.02740 source file (2024-06-04)
Supplement: Supplementary file 5 [file appendix_time_vs_nparams.tex]

% This table is just for reference. Instead of this we will make a plot
                 &                time &  dim & nlayer &  params \\
DyRep            &   28.31$_{\pm0.82}$ &   63 &      1 &   49991 \\
DyRep            &   30.06$_{\pm0.33}$ &   96 &      1 &   98451 \\
DyRep            &   33.91$_{\pm1.29}$ &  123 &      1 &  149261 \\
DyRep            &   36.55$_{\pm1.17}$ &  145 &      1 &  198288 \\
DyRep            &    38.46$_{\pm0.4}$ &  165 &      1 &  248738 \\

JODIE            &   23.22$_{\pm0.53}$ &   89 &      1 &   49118 \\
JODIE            &   24.88$_{\pm0.71}$ &  135 &      1 &   99327 \\
JODIE            &   27.05$_{\pm1.21}$ &  170 &      1 &  149042 \\
JODIE            &   29.06$_{\pm0.83}$ &  200 &      1 &  199337 \\
JODIE            &   31.46$_{\pm0.99}$ &  226 &      1 &  248750 \\

TGAT$_{1L}$      &   15.47$_{\pm0.31}$ &   87 &      1 &   49230 \\
TGAT$_{1L}$      &   20.58$_{\pm0.49}$ &  145 &      1 &   98849 \\
TGAT$_{1L}$      &   24.26$_{\pm0.66}$ &  192 &      1 &  149313 \\
TGAT$_{1L}$      &   29.47$_{\pm0.67}$ &  233 &      1 &  199829 \\
TGAT$_{1L}$      &   31.27$_{\pm0.54}$ &  268 &      1 &  249139 \\

TGAT$_{5L}$      &   54.94$_{\pm1.58}$ &   16 &      5 &   47929 \\
TGAT$_{5L}$      &   69.21$_{\pm1.03}$ &   26 &      5 &   94944 \\
TGAT$_{5L}$      &   79.18$_{\pm1.57}$ &   35 &      5 &  148472 \\
TGAT$_{5L}$      &   89.44$_{\pm2.68}$ &   42 &      5 &  197624 \\
TGAT$_{5L}$      &   90.54$_{\pm0.61}$ &   48 &      5 &  244841 \\

TGN$_{1L}$       &   25.82$_{\pm0.43}$ &   31 &      1 &   48097 \\
TGN$_{1L}$       &   28.55$_{\pm0.73}$ &   51 &      1 &   98487 \\
TGN$_{1L}$       &   31.31$_{\pm0.71}$ &   67 &      1 &  149743 \\
TGN$_{1L}$       &   34.18$_{\pm0.61}$ &   80 &      1 &  198713 \\
TGN$_{1L}$       &   36.88$_{\pm0.75}$ &   92 &      1 &  249491 \\

TGN$_{5L}$       &   74.69$_{\pm2.09}$ &   13 &      5 &   46526 \\
TGN$_{5L}$       &   82.79$_{\pm1.75}$ &   22 &      5 &   95194 \\
TGN$_{5L}$       &   92.99$_{\pm1.33}$ &   30 &      5 &  149718 \\
TGN$_{5L}$       &  100.78$_{\pm1.99}$ &   36 &      5 &  197583 \\
TGN$_{5L}$       &  108.35$_{\pm1.75}$ &   41 &      5 &  241952 \\

Our$_{1L}$       &   14.85$_{\pm0.69}$ &   71 &      1 &   49199 \\
Our$_{1L}$       &   16.65$_{\pm0.53}$ &  106 &      1 &   99514 \\
Our$_{1L}$       &   20.46$_{\pm0.89}$ &  133 &      1 &  149856 \\
Our$_{1L}$       &   21.32$_{\pm0.79}$ &  155 &      1 &  198509 \\
Our$_{1L}$       &   27.18$_{\pm2.76}$ &  175 &      1 &  248619 \\

Our$_{5L}$       &   78.22$_{\pm2.27}$ &   71 &      5 &   49199 \\
Our$_{5L}$       &  101.71$_{\pm0.89}$ &  106 &      5 &   99514 \\
Our$_{5L}$       &  125.43$_{\pm2.12}$ &  133 &      5 &  149856 \\
Our$_{5L}$       &  147.08$_{\pm2.54}$ &  155 &      5 &  198509 \\
Our$_{5L}$       &  161.61$_{\pm2.77}$ &  175 &      5 &  248619 \\

Our(tanh)$_{1L}$ &   13.98$_{\pm0.24}$ &   71 &      1 &   49199 \\
Our(tanh)$_{1L}$ &   16.64$_{\pm0.56}$ &  106 &      1 &   99514 \\
Our(tanh)$_{1L}$ &   19.15$_{\pm0.45}$ &  133 &      1 &  149856 \\
Our(tanh)$_{1L}$ &   21.38$_{\pm0.58}$ &  155 &      1 &  198509 \\
Our(tanh)$_{1L}$ &   22.68$_{\pm0.41}$ &  175 &      1 &  248619 \\

Our(tanh)$_{5L}$ &   77.35$_{\pm1.21}$ &   71 &      5 &   49199 \\
Our(tanh)$_{5L}$ &   102.0$_{\pm1.88}$ &  106 &      5 &   99514 \\
Our(tanh)$_{5L}$ &   127.4$_{\pm2.88}$ &  133 &      5 &  149856 \\
Our(tanh)$_{5L}$ &  144.18$_{\pm2.51}$ &  155 &      5 &  198509 \\
Our(tanh)$_{5L}$ &  158.07$_{\pm4.97}$ &  175 &      5 &  248619 \\
